# Supplementary material for: Universal Scaling of Electron Transmission for Nearly Ballistic and Quantum Dragon Nanodevices
Source: arXiv:2007.01051 ancillary file (2025-12-29)
Supplement: Supplementary file 1 [file PRR_Dragon_Supplemental_2020_arXiv.pdf]

# Order amidst disorder in semi-regular, tatty, and atypical random nanodevices with locally correlated disorder

## Supplemental Material

M.A. Novotny  
*Department of Physics and Astronomy*  
*HPC<sup>2</sup> Center for Computational Sciences*  
*Mississippi State University*  
*Mississippi State, MS 39762-5167\**

Tomáš Novotný  
*Department of Condensed Matter Physics*  
*Faculty of Mathematics and Physics*  
*Charles University*  
*Ke Karlovu 5*  
*CZ-121 16 Prague, Czech Republic*  
(Dated: July 1, 2020)

Supplemental material includes additional figures, `.cdf` files, and descriptions for the additional figures and `.cdf` files. The `.cdf` files allow manipulations for different parameter values, as well as the ability to modify viewpoints in 3D graphics.

---

### INTRODUCTION TO SUPPLEMENTAL MATERIAL

The main point of the supplemental material is to provide example 2D, 3D, and 2D+3D nanodevices related to those presented in the main article. The nanodevice models were constructed using Mathematica [1]. The models, using a ball-and-stick model for the atomic arrangements and bonds, are presented as separate files using the Wolfram `.cdf` data format. This is the Wolfram Computable Document Format (CDF). It is an ASCII format utilized as a deployment format for interactive use in the Wolfram Player. A free Wolfram CDF Player is available for Windows, Mac, Linux, as well as for iOS for iPad and iPhone. Important aspects of the presentation:

- Pop-up buttons are used to set the values for the various parameters.
  - Care must be taken not to overwhelm the computing power of your electronic device. This should be taken as a consideration particularly when choosing a large nanodevice or a large number of energies  $E$  at which to calculate the transmission  $\mathcal{T}(E)$ .
- The plots and 3D graphics can be resized by ‘grabbing’ a corner to make it larger.
- The 3D graphics can be ‘clicked’ in order to change the viewpoint.

Table I describes the four `.cdf` files that allow for contents to be manipulated, and each has a section below that can be a ‘user manual’ for the program. The ten `.cdf` files allowing viewpoint changes in 3D graphs from the main paper are listed in Table VIII.

---

\* man40@msstate.edu

The nanodevices presented in the `.cdf` files using a Mathematica call to **Manipulate** typically have a smaller number of atoms than those in the main paper. This should allow enhanced interactivity even on devices that have smaller memory and limited bandwidth.

Table I. Overview of the four `.cdf` files that allow for manipulation of variables.

| File Name               | Purpose                                                                                                                  | Brief Description                                  |
|-------------------------|--------------------------------------------------------------------------------------------------------------------------|----------------------------------------------------|
| Dragon_cdf1_NanoTube    | To show: $\begin{cases} \bullet \text{ SWNT quantum dragons} \\ \bullet \text{ Nearly quantum dragon SWNTs} \end{cases}$ | $\ell \times m$ SWNTs based on 2D hexagonal graphs |
| Dragon_cdf2_FindDragons | To illustrate how to find quantum dragons                                                                                | $\ell \times m$ SWNTs based on 2D hexagonal graphs |
| Dragon_cdf3_Cdevice     | To illustrate single walled dragons, 2D $\rightarrow$ 3D                                                                 | $\ell \times m$ based on 2D hexagonal nanoribbons  |
| Dragon_cdf4_0aD         | To demonstrate <b>Order amidst Disorder</b>                                                                              | $\ell \times m$ based on 2D hexagonal nanoribbons  |

Here the acronyms include:

- SWNT : Single-Walled NanoTube
- 2D : Two dimensional
- 3D : Three dimensional

The Hamiltonian for an  $\ell$  slice device is given as in the main paper by

$$\mathcal{H}_\ell = \sum_{j=1}^{\ell} \sum_{i=1}^m \epsilon_{i,j} \hat{c}_{i,j}^\dagger \hat{c}_{i,j} - \sum_{\langle i,j;i',j' \rangle} t_{i,j;i',j'} \left( \hat{c}_{i,j}^\dagger \hat{c}_{i',j'} + \hat{c}_{i',j'}^\dagger \hat{c}_{i,j} \right). \quad (1)$$

The first sum is over all  $N = m\ell$  atoms of the nanomaterial. Every on site energy can have its own value  $\epsilon_{i,j}$ , and the first sum is over all  $N$  atoms. The second sum is over all edges (or bonds) of the  $N$  vertex graph. Every bond can have its own bond strength  $t_{i,j;i',j'}$ . The graph with  $\ell$  slices are constrained to have two types of bonds:

- **Intra-** : intra-slice bonds which have  $j' = j$  and a nearest-neighbor constraint  $i' = i \pm 1$ . Thus  $t_{i,j;i\pm 1,j}$  are the bond strengths.
- **Inter-** : inter-slice bonds which have  $j' = j \pm 1$  and a nearest neighbor ( $i' = i$ ) and 2<sup>nd</sup> neighbor ( $i' = i \pm 1$ ) constraint. Thus  $t_{i,j;i',j\pm 1}$  are the bond strengths.

### I. CDF#1: 2D HEXAGONAL NANOTUBE $\mathcal{T}(E)$

In order to illustrate the transmission  $\mathcal{T}(E)$ , the .cdf file `Dragon_cdf1_Nanotube.cdf` is available. The user can adjust 7 dropdown variables for the nanodevice, as shown in Table II. It is easy to overwhelm the computational power of your device, and therefore the initial values are for relatively small values for  $\ell$ ,  $m$ , and the number of energy points.

Table II. Description of the `Dragon_cdf1_NanoTube.cdf` seven popup variables for the nanodevice.

|                                         |                                                                                                                                                                                                                                         |
|-----------------------------------------|-----------------------------------------------------------------------------------------------------------------------------------------------------------------------------------------------------------------------------------------|
| $\ell = \# \text{ slices:}$             | Number of slices $\ell$                                                                                                                                                                                                                 |
| $m = \# \text{ atoms per slice:}$       | Number of atoms per slice, $m$                                                                                                                                                                                                          |
| $\Delta_{\text{Dragon},A}:$             | The intra-slice bond strengths are chosen uniformly at random<br>with $t_{i,j;i+1,j} \in [1 - \Delta_{\text{Dragon},A}, 1 + \Delta_{\text{Dragon},A}]$                                                                                  |
| $\delta:$                               | Uncorrelated additional on site disorder, added to the dragon on site energy via<br>$\epsilon_{i,j} \rightarrow \epsilon_{i,j} + \delta_{i,j}$ with each randomly chosen value uniformly picked in $\delta_{i,j} \in [-\delta, \delta]$ |
| $\# \text{ cuts:}$                      | Number of cuts along the electron flow axis, with the cut randomly chosen between<br>$i_{\text{cutleft}} \in [1, \ell/2]$ and $i_{\text{cutright}} \in [\ell/2, \ell]$                                                                  |
| <code>fraction intra- bonds = 0:</code> | Fraction of intra-slice bonds randomly, independently set to zero (before the cuts are put in)                                                                                                                                          |
| $\# E \text{ points:}$                  | Number of energy points to calculate, from $E_{\min} = -1.999$ to $E_{\max} = 1.999$                                                                                                                                                    |

An example of the output is shown in Fig. 1. This is an example with no added on site disorder ( $\delta = 0$ ), together with  $\ell = 24$ ,  $m = 12$ ,  $\Delta_{\text{Dragon}} = 0.5$  with one cut and 16 energy points. The output of the .cdf includes three graphs, with an example in Fig. 1.

- **TOP:** This figure shows the nanodevice, drawn as a SWNT (Single Wall NanoTube). This is the type of tube carbon-based materials form. This top figure illustrates the disorder nanodevice. The on site energies are depicted as spheres with radii proportional to  $|\epsilon_{i,j}|$ , with red spheres for  $\epsilon_{i,j} > 0$  and black spheres for  $\epsilon_{i,j} < 0$ . If  $\epsilon_{i,j} = 0$  a yellow sphere is shown. The bond strengths  $t_{i,j;i',j'}$  are shown as being proportional to the radii of the cyan cylinders. The device illustration shows 3 lead atoms of the semi-infinite left lead and 2 lead atoms of the semi-infinite right lead. This 3D graphic can have the viewpoint changed by clicking into the frame and using mouse/touch-pad input.
- **MIDDLE:** The transmission  $\mathcal{T}(E)$  is shown (red points) for calculated energy values. For comparison there is a green semi-transparent line drawn for  $\mathcal{T}(E) = 1$ . Note because  $\mathcal{T}(E)$  is a transmission probability, it must be bounded as  $0 \leq \mathcal{T}(E) \leq 1$ .
- **BOTTOM:** The result of the Mathematica call `GraphPlot3D[ $\mathcal{H}_\ell$ ]`, where the Hamiltonian  $\mathcal{H}_\ell$  (with no leads attached) is a  $N \times N$  (with  $N = m\ell$ ) matrix. This shows the disorder in the graph of the nanomaterial. It is possible to change the viewpoint of this 3D graph.

The nanodevices here have uniform inter-slice interactions, namely all  $\mathbf{B}_{j,j+1} = -\mathbf{I}_{m \times m}$ . They also use a uniform  $\vec{v}_{\text{Dragon}}$ , with every element equal to  $m^{-\frac{1}{2}}$ . If  $\delta = 0$  every on site energy satisfies the dragon condition  $\epsilon_{i,j} = t_{i,j;i-1,j} + t_{i,j;i+1,j}$  so for all calculated energies  $\mathcal{T}(E) = 1$ .

Running the file `Dragon_cdf1_NanoTube.cdf` allows one to show an ordered nanodevice with ballistic electron propagation ( $\mathcal{T}(E) = 1$ ) if  $\Delta_{\text{Dragon},A} = \delta = 0$ , with no cuts or intra-slice bonds set to zero. It is possible to show a quantum dragon ( $\mathcal{T}(E) = 1$ ) if one keeps  $\delta = 0$  while putting on a few cuts, setting a non-zero  $\Delta_{\text{Dragon},A}$ , setting a fraction of intra-slice bonds to zero, or any combination. The dragon condition is always set, namely  $\epsilon_{i,j} = t_{i,j;i+1,j} + t_{i,j;i-1,j}$ , with at most one of these intra-slice bonds non-zero (due to the underlying armchair 2D hexagonal graph). In order to not have unit transmission one can set  $\delta \neq 0$ .

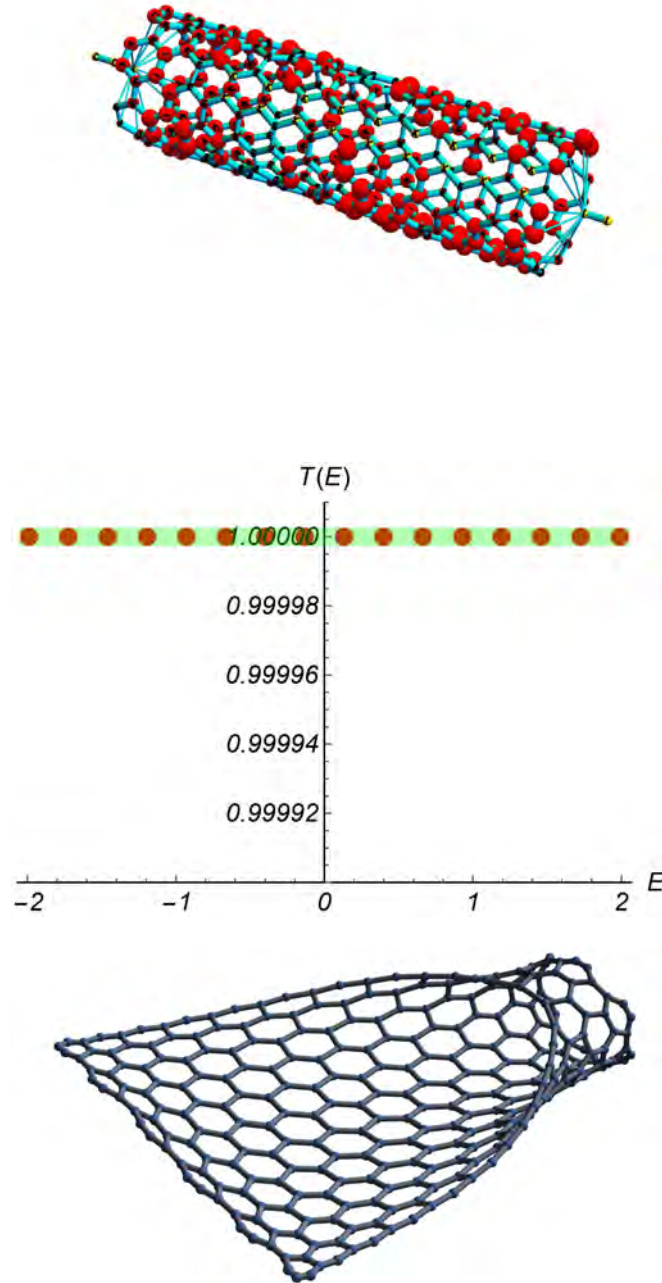

Figure 1. Example output from `Dragon_cdf1_NanoTube.cdf`. See the text in Sec. I for a complete description.

## II. CDF#2: UNITARY TRANSFORMATION FOR NANODEVICES

The purpose of the file `Dragon_cdf2_FindDragon.cdf` is to illustrate the unitary transformation that enables a person for atypical disorder to find a quantum dragon. The underlying graph is based on an armchair hexagonal SWNT, with  $\ell$  slices and  $m$  vertices in each slice. The True-False (T-F) controls are listed in Table III and the popup controls in Table IV. The 3D graphics can be manipulated by double-clicking in the graphic frame and using mouse/touchpad controls to rotate the graphic. (Note: if you see a blank screen your viewing window is too narrow.)

The Hamiltonian  $\mathcal{H}_\ell$  is composed of two parts. The first is the device Hamiltonian for a quantum dragon,  $\mathcal{H}_{\text{Dragon}}$ . There is atypical, locally correlated disorder in  $\mathcal{H}_{\text{Dragon}}$ . The second is the uncorrelated disorder of strength  $\delta$  for the on site values  $\epsilon_{i,j}$ , forming an  $N \times N$  diagonal matrix  $\mathcal{H}_\delta$  with each diagonal value chosen uniformly in  $[-\delta, \delta]$ . The total device Hamiltonian is  $\mathcal{H}_\ell = \mathcal{H}_{\text{Dragon}} + \mathcal{H}_\delta$ , which is used to calculate the transmission  $\mathcal{T}(E)$  and the change of basis (mapped) Hamiltonian  $\mathcal{H}_{\text{map}} = \mathbf{U}_N^\dagger \mathcal{H}_\ell \mathbf{U}_N$  with unitary  $N \times N$  matrix  $\mathbf{U}_N$ . The dragon device has a uniform  $\vec{v}_{\text{Dragon}}$  with every element equal to  $1/\sqrt{m}$ .

Table III. Description of the `Dragon_cdf2_FindDragon.cdf` seven check-box controls.

|     |                                                                |                                                                                                                                                                                                                                                                                                                                                               |
|-----|----------------------------------------------------------------|---------------------------------------------------------------------------------------------------------------------------------------------------------------------------------------------------------------------------------------------------------------------------------------------------------------------------------------------------------------|
| T-F | New Dragon $\mathcal{H}$                                       | If checked a new device Hamiltonian $\mathcal{H}_{\text{Dragon}}$ is calculated when popup values are changed. The Hamiltonian is set to the dragon condition, so the it shows <b>order amidst disorder</b> and $\mathcal{T}(E) = 1$ for $-2 < E < 2$ .<br>A new Hamiltonian is also calculated whenever popup menus change values for either $\ell$ or $m$ . |
| T-F | New $\delta$ disorder                                          | If unchecked and re-checked new uncorrelated random disorder with strength $\delta$ is formed.                                                                                                                                                                                                                                                                |
| T-F | <b>Plot/Eval:</b> Devices                                      | Plot, if checked, as a ball-and-stick model both the device Hamiltonian $\mathcal{H}_\ell$ in physical space and in the new basis after the unitary transformation by $\mathbf{U}_N$ gives $\mathcal{H}_{\text{map}}$ .                                                                                                                                       |
| T-F | <b>Plot/Eval:</b> $\mathcal{T}(E)$                             | Calculate and plot, if checked, $\mathcal{T}(E)$ for the select number of energies.                                                                                                                                                                                                                                                                           |
| T-F | <b>Plot/Eval:</b> Graphs                                       | Plot if checked the graphs, using <code>GraphPlot3D[H]</code> for both the physical $\mathcal{H}_\ell$ and after the unitary transformation <code>GraphPlot3D[U<sub>N</sub><sup>†</sup> <math>\mathcal{H}_\ell</math> <math>\mathbf{U}_N</math>].<br/>Both shown with 3 (2) atoms in the left (right) semi-infinite lead.</code>                              |
| T-F | <b>Plot/Eval:</b> X,P,U                                        | If checked a matrix plot of the transformation matrix $\mathbf{X}_N$ , the permutation matrix $\mathbf{P}_N$ , and the total unitary transformation matrix $\mathbf{U}_N = \mathbf{X}_N \mathbf{P}_N$ are shown.                                                                                                                                              |
| T-F | <b>Plot/Eval:</b> $\mathcal{H}$ and $\mathcal{H}_{\text{map}}$ | If checked a matrix plot for both $\mathcal{H}_\ell$ and $\mathcal{H}_{\text{map}}$ are shown.                                                                                                                                                                                                                                                                |

Table IV. Description of the `Dragon_cdf2_FindDragon.cdf` eight popup variable controls. Note  $i \pm 1$  is to be read including periodic boundary conditions, so  $i+1 \rightarrow 1$  for  $i=m$  and  $i-1 \rightarrow m$  for  $i=1$ .

|                                   |                                                                                                                                                                                                                                                                                              |
|-----------------------------------|----------------------------------------------------------------------------------------------------------------------------------------------------------------------------------------------------------------------------------------------------------------------------------------------|
| $\ell = \# \text{ slices:}$       | Number of slices $\ell$ .                                                                                                                                                                                                                                                                    |
| $m = \# \text{ atoms per slice:}$ | Number of atoms per slice, $m$ . Here $m = 2^n$ .                                                                                                                                                                                                                                            |
| $\Delta_{\text{Dragon},A}:$       | The intra-slice bond strengths are chosen uniformly at random<br>with $t_{i,j;i+1,j} \in [1 - \Delta_{\text{Dragon},A}, 1 + \Delta_{\text{Dragon},A}]$ on the armchair hexagonal SWNT.                                                                                                       |
| $\Delta_{\text{Dragon},B}:$       | The inter-slice bond strengths are chosen uniformly at random. Let $r_j \in [1 - \Delta_{\text{Dragon},B}, 1]$ .<br>All $m$ inter-slice nearest-neighbor bonds have bond strength $t_{i,j;i,j+1} = r_j$ , while<br>all $2m$ next-nearest neighbors have $t_{i,j;i\pm 1,j+1} = (1 - r_j)/2$ . |
| $\delta:$                         | Uncorrelated additional on site disorder, added to the dragon on site energy via<br>$\epsilon_{i,j} \rightarrow \epsilon_{i,j} + \delta_{i,j}$ with the random value $\delta_{i,j} \in [-\delta, \delta]$                                                                                    |
| $\# \text{ cuts:}$                | Number of cuts along the electron flow axis, with the cut randomly chosen between<br>$i_{\text{cut, left}} \in [1, \ell/2]$ and $i_{\text{cut, right}} \in [\ell/2, 1]$ . No cuts on inter-slice bonds.                                                                                      |
| <b>fraction intra- bonds = 0:</b> | Fraction of intra-slice bonds set uniformly at random to zero (before the cuts are put in)                                                                                                                                                                                                   |
| $\# E \text{ points:}$            | Number of energy points to calculate, from $E_{\min} = -1.999$ to $E_{\max} = 1.999$                                                                                                                                                                                                         |

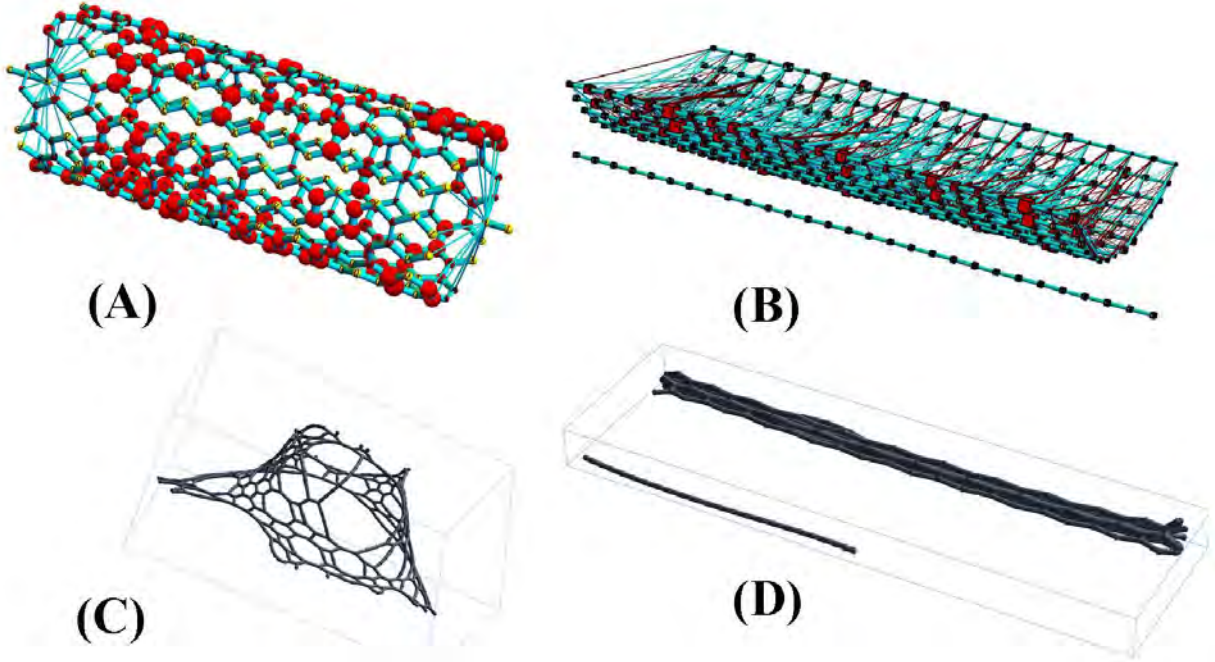

Figure 2. A quantum dragon nanodevice with  $\ell = 24$ ,  $m = 16$ ,  $\Delta_{\text{Dragon,A}} = 0.5$ ,  $\Delta_{\text{Dragon,B}} = 0$ ,  $\delta = 0$ ,  $\#_{\text{cuts}} = 2$ , and  $f_{\text{intra-bonds}=0} = 0.3$ . In physical space the device Hamiltonian  $\mathcal{H}_{24}$  is shown in (A) and the graph in (C). In the mapped space the device Hamiltonian  $\mathcal{H}_{\text{map}}$  is depicted in (B) and the graph in (D). Here  $N = \ell m = 384$ .

An example of a constructed quantum dragon nanodevice from this `Dragon_cdf2_FindDragon.cdf` program is shown in Fig. 2. The device in physical space, with Hamiltonian  $\mathcal{H}_{24}$  has locally-correlated (atypical) disorder shown in Fig. 2(A), and the underlying disordered graph is shown in Fig. 2(C). In the mapped space with Hamiltonian  $\mathcal{H}_{\text{map}}$  the associated figures are in Fig. 2(B) and Fig. 2(D), respectively. Note in Fig. 2(B) and Fig. 2(D) the fact that the device has a uniform length  $\ell = 24$  wire piece disconnected from a disordered piece with  $(\ell - 1)m = 360$  atoms. In Fig. 2(A) and (B) vertices with  $\epsilon_{i,j}=0$  are depicted by yellow spheres, which include the lead atoms. In Fig. 2(A) the red (black) spheres have  $\epsilon_{i,j} > 0$  ( $\epsilon_{i,j} < 0$ ), with radii proportional to  $|\epsilon_{i,j}|$ . In Fig. 2(B) the red (black) cubes have  $\epsilon_{i,j} > 0$  ( $\epsilon_{i,j} < 0$ ), with size proportional to  $|\epsilon_{i,j}|$ . In Fig. 2(A) and (B) the cyan (maroon) cylinders depict bonds with hopping  $t_{i,j;i',j'} > 0$  ( $t_{i,j;i',j'} < 0$ ), with cylinder radii proportional to  $|t_{i,j;i',j'}|$ . In Fig. 2(B) the vertices are laid out in a fashion that does not depict real space, except for the axis along which the electrons flow. Note in particular in Fig. 2(B) and (D) the uniform linear subgraphs with  $\ell = 24$  atoms, making clear the device is a quantum dragon with  $\mathcal{T}(E) = 1$ .

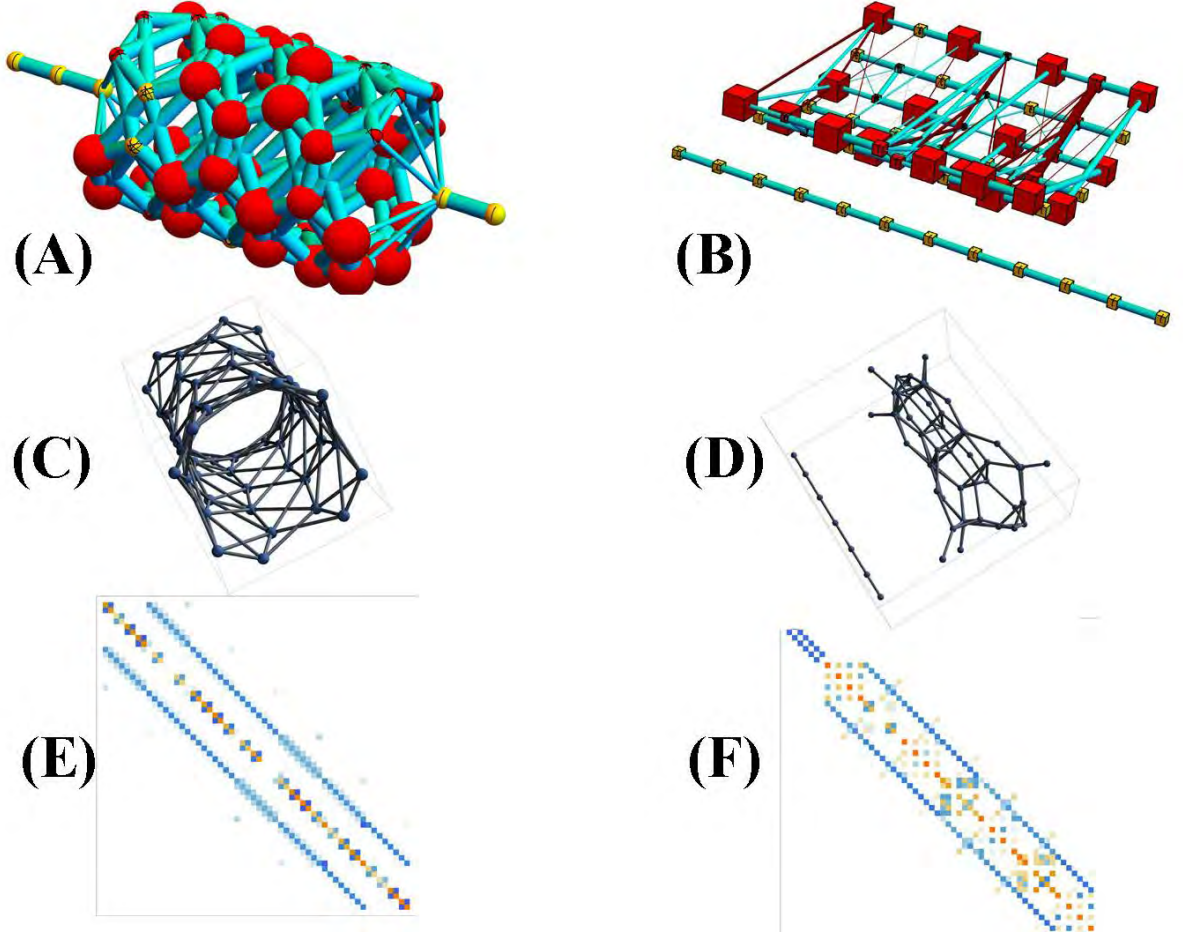

Figure 3. A quantum dragon nanodevice with  $\ell = 7$ ,  $m = 8$ ,  $\Delta_{\text{Dragon,A}} = 0.5$ ,  $\Delta_{\text{Dragon,B}} = 0.5$ ,  $\delta = 0$ ,  $\#_{\text{cuts}} = 0$ , and  $f_{\text{intra-bonds}=0} = 0.1$ . In physical space the device is shown in (A), the graph in (C), and the Hamiltonian  $\mathcal{H}_7$  in (E). In the mapped space the device is shown in (B), the graph in (D), and the Hamiltonian  $\mathcal{H}_{\text{map}}$  in (F). Here  $N = \ell m = 56$ .

An example of a constructed quantum dragon nanodevice and its Hamiltonian from the `Dragon_cdf2_FindDragon.cdf` file is shown in Fig. 3. The device in physical space, with Hamiltonian  $\mathcal{H}_7$  has locally-correlated (atypical) disorder shown in Fig. 3(A) on a disordered underlying graph shown in Fig. 3(C), and block-tri-diagonal Hamiltonian  $\mathcal{H}_7$  in Fig. 3(E). In the mapped space with Hamiltonian  $\mathcal{H}_{\text{map}}$  the associated figures are in Fig. 3(B), Fig. 3(D), and Fig. 2(F), respectively. Note in particular in Fig. 3(B), (D), and (F) the uniform linear subgraphs with  $\ell = 7$  atoms, making clear the device is a quantum dragon with  $\mathcal{T}(E) = 1$  and **order amidst disorder**. In particular, in Fig. 3(F) the top-right  $7 \times 7$  submatrix is that for a uniform wire.

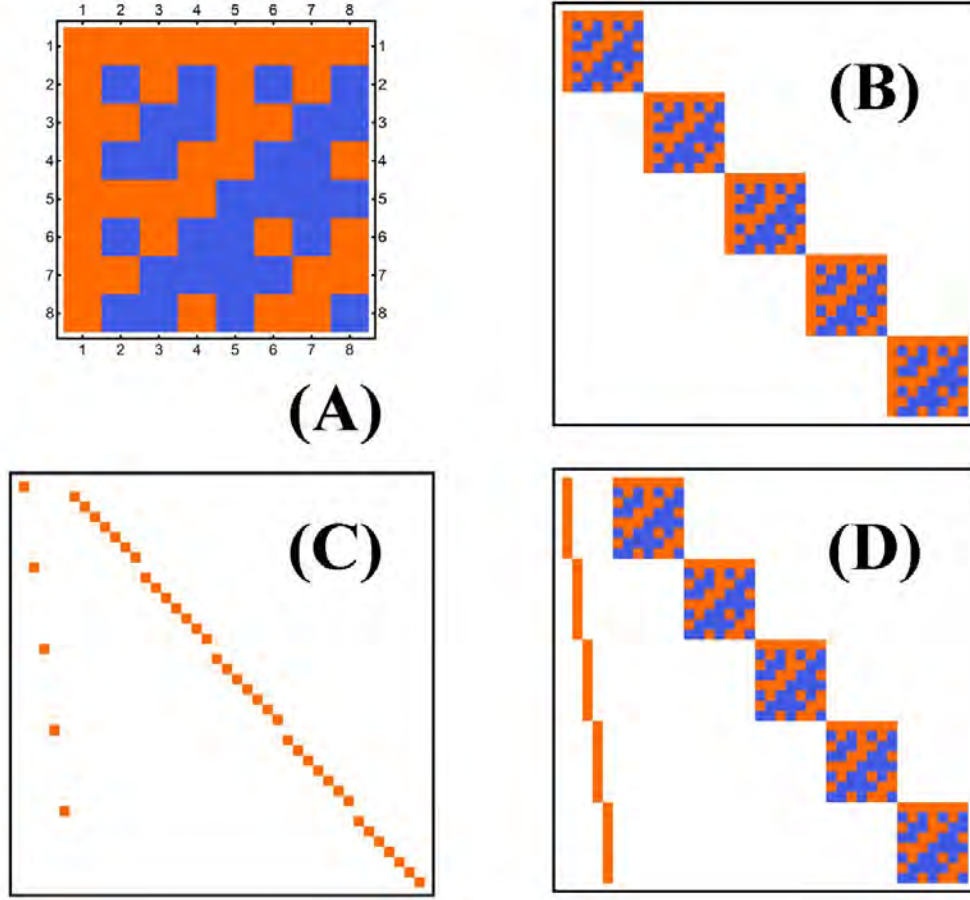

Figure 4. An example of the unitary transformation matrix construction to find a quantum dragon nanodevice with  $\ell = 5$  and  $m = 8$ , so  $N = \ell m = 40$ . (A) shows the  $m \times m$  matrix  $\mathbf{Y}_{8 \times 8}$ . (B) shows the  $N \times N$  unitary matrix  $\mathbf{X}_N$ . (C) shows the  $N \times N$  permutation matrix  $\mathbf{P}_N$ . (D) shows the  $N \times N$  unitary matrix  $\mathbf{U}_N = \mathbf{X}_N \mathbf{P}_N$ .

Fig. 4 shows the transformation matrix for any nanodevice with  $\ell = 5$  and  $m = 8$ . The same transformation matrix is used regardless of the disorder values, as long as one has a uniform  $\vec{v}_{\text{Dragon}}$  vector.

First introduce the matrix  $Y_{2 \times 2} = \frac{1}{\sqrt{2}} \begin{pmatrix} 1 & 1 \\ 1 & -1 \end{pmatrix}$ . For any nanodevice with  $m = 2^n$  the  $2^n \times 2^n$  matrix  $\mathbf{Y}_{2^n \times 2^n}$  is formed by the Kronecker matrix product of  $\mathbf{Y}_{2 \times 2}$  with itself  $n$  times. An example for  $n = 3$  (so  $m = 8$ ) is shown in Fig. 4(A). Here the orange (blue) color denotes the value  $+2^{-n/2}$  ( $-2^{-n/2}$ ). The text describes use of a  $m \times m$  matrix using a length  $m$  discrete Fourier transform matrix. However, that leads to complex elements in  $\mathcal{H}_{\text{map}}$ , thereby making plotting difficult. That is why here we choose  $\mathbf{Y}_{2^n \times 2^n}$  to be real, while it is also unitary. Note the first row and the first column of  $\mathbf{Y}_{m \times m}$  is  $\vec{v}_{\text{Dragon}}$ .

Fig. 4(B) shows the block-tri-diagonal unitary matrix  $\mathbf{X}_N$ , with  $\ell$  blocks each of which is  $\mathbf{Y}_{m \times m}$ .

Fig. 4(C) shows the  $N \times N$  permutation matrix  $\mathbf{P}_N$ . Here the orange squares are equal to unity. The goal of  $\mathbf{P}_N$  is to pick out the first element in each of the  $\ell$  blocks and put them into the first  $\ell$  vertices.

Fig. 4(D) shows the  $N \times N$  total unitary matrix  $\mathbf{U}_N = \mathbf{X}_N \mathbf{P}_N$ .

Some examples of the tight binding model, based on 2D hexagonal graphs, are shown in the `.cdf` program

0aD\_TB\_map.cdf (based on a SWNT) and Fig. ???. Figure ?? is based on a 2D hexagonal nanoribbon, and includes also random next-nearest neighbor intra-slice (constrained to neighboring slices) bonds. Figure ?? and the 0aD\_TB\_map.cdf file show both the real-space nanodevice as well as the nanodevice in the transformed basis. For a nanodevice with  $\ell$  slices and  $N$  atoms the  $N \times N$  unitary matrix  $\mathbf{X}_\ell$  is introduced, with  $\mathbf{X}_\ell^\dagger \mathbf{X}_\ell = \mathbf{I}$  with  $\mathbf{I}$  the  $N \times N$  identity matrix. There are four possibilities when one tries a unitary transformation  $\mathbf{X}_\ell$  on the Hamiltonian  $\mathcal{H}$  of an  $\ell$ -slice nanodevice

$$\mathcal{H}_{\text{map}} = \mathbf{X}_\ell^\dagger \mathcal{H}_\ell \mathbf{X}_\ell \quad (2)$$

with  $\mathcal{H}$  the real-space Hamiltonian of Eq. (??). These are shown as

- Fig. ??(a): There is no special structure in  $\mathcal{H}_{\text{map}}$ , so every site is still part of a connected graph, which is connected to the semi-infinite leads.
- Fig. ??(b): There is a disconnect between the 1D graph attached to the semi-infinite leads and the rest of the mapped graph. This happens when every one of the  $m \times m$  matrices  $\mathbf{A}_j$  and  $\mathbf{B}_{j,j+1}$  have a common eigenvector, but these eigenvectors have eigenvalues that depend on the slice index  $j$ . This leads to transmission being that of a 1D disordered system, with for almost every energy  $\mathcal{T}(E) \ll 1$ .
- Fig. ??(c): The transformed (mapped) Hamiltonian yields a quantum dragon ( $\mathcal{T}(E) = 1$  for  $-2 < E < 2$ ) and **order amidst disorder**. The graph attached to the semi-infinite leads is a 1D uniform wire with  $\ell$  atoms. This happens when all  $\mathbf{A}_j$  have a common eigenvector which all have a common eigenvalue of zero, and all  $\mathbf{B}_{j,j+1}$  have the same common eigenvector with eigenvalue which has an absolute value of unity.
- Fig. ??(d): By adding a small amount of uncorrelated disorder to Fig. ??(c), one is near a quantum dragon solution. Again every atom is part of the connected graph of the semi-infinite leads, but there is weak coupling between the 1D wire part and the formerly disconnected part.

By eye it is very difficult to determine which of these possibilities a disordered nanodevice will fall into. The typical disorder will be as in as in Fig. ??(a), while the atypical disorder yields very interesting physical behavior. There are, of course, other possibilities, for example if the 1D wire is connected to the wrong type or in the wrong way of the semi-infinite leads.

Figure 5 shows four examples of the possibilities of using the mapping performed by the similarity transformation:

- (a) In the transformed basis the system is still very disordered, and therefore for typical disorder the transformation does not help analysis.
- (b) In the transformed basis the system has a 1D wire disconnected from the rest, but the wire is disordered and hence will show Anderson localization effects.
- (c) In the transformed basis one finds a **quantum dragon**, with a uniform wire connected to the leads and disconnected from the rest of the degrees of freedom. Thus the system has **order amidst disorder** and  $\mathcal{T}(E) = 1$  for all energies in  $-2 < E < 2$ .
- (d) In the transformed basis the wire is almost uniform, and is only weakly connected to the other degrees of freedom. Therefore the disorder is ‘close to being a quantum dragon’ (the disorder is very near to the dragon’s den).

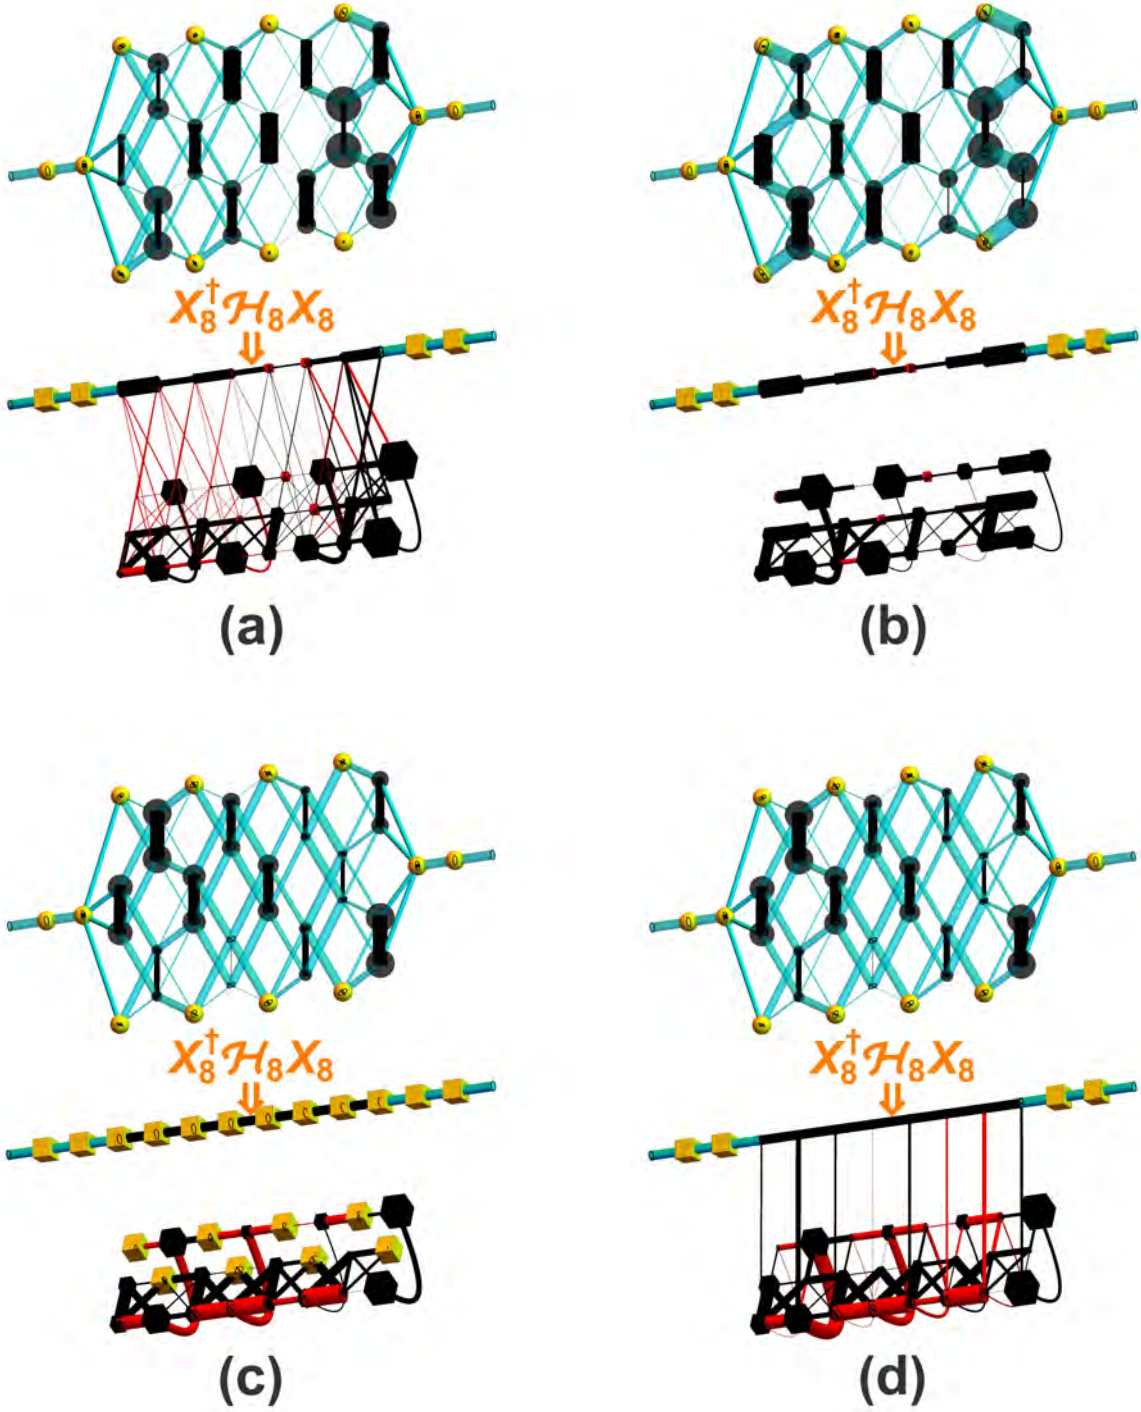

Figure 5. Four examples of performing a unitary transformation on the Hamiltonian  $\mathcal{H}$ . See text for full description.

### III. CDF#3: QUANTUM DRAGONS BASED ON 2D HEXAGONAL GRAPHS

The purpose of this `.cdf` program is to illustrate quantum dragon nanodevices based on the allowed manipulations of:

- Cutting
- Sewing (or stitching)
- Twisting
- Braiding

based on an underlying graphene nanoribbon (GNR). Thus we only present the underlying graphs, based on an underlying 2D hexagonal graph with only nn bonds, that allow quantum dragons. We do not actually invoke the Hamiltonian, we only study the underlying graph (vertices and edges — atoms and bonds). Due to the 2D hexagonal graph, every atom in the bulk of the device has one inter-slice bond  $t_{i,j;i,j+1}$  and has either zero or one intra-slice bonds  $t_{i,j;i+1,j}$  (neglecting atoms that connect to the leads).

It is possible to *just play* with this `.cdf` program, maybe with the help of the variable descriptions in Table V.

Table V. Description of the `Dragon_cdf3_Cdevice.cdf` popup variable controls. Note  $i \pm 1$  is to be read including periodic boundary conditions, so  $i+1 \rightarrow 1$  for  $i=m$  and  $i-1 \rightarrow m$  for  $i=1$ . The last column recalculates the entire Hamiltonian if ‘Yes’ and the value is changed, using new random numbers for random missing intra-slice bonds and randomly performed ribbon braiding.

|                                         |                                                                                           |     |
|-----------------------------------------|-------------------------------------------------------------------------------------------|-----|
| $\ell = \# \text{ slices:}$             | Number of slices $\ell$                                                                   | Yes |
| $m = \# \text{ atoms per slice:}$       | Number of atoms per slice, $m$ (here $m$ even)                                            | Yes |
| $\# \text{ left lead atoms:}$           | Number of left lead atoms to include in graph                                             | Yes |
| $\# \text{ right lead atoms:}$          | Number of right lead atoms to include in graph                                            | Yes |
| <code>fraction intra- bonds = 0:</code> | Fraction intra-slice bonds set uniformly at random to zero                                | Yes |
| $\# \text{ Left to sew:}$               | Sew into tube this $\#$ left-hand columns                                                 | No  |
| $\# \text{ Right to sew:}$              | Sew into tube this $\#$ right-hand columns                                                | No  |
| $i\text{Cut}\#1:$                       | Bond $i \leftrightarrow i + 1$ for cut $\#1$ ( $= 0$ for no cut)                          | No  |
| $j \text{ Left Cut}\#1:$                | Column $\#$ to start cut $\# 1$                                                           | No  |
| $j \text{ Right Cut}\#1:$               | Column $\#$ to end cut $\# 1$                                                             | No  |
| $i\text{Cut}\#2:$                       | Bond $i \leftrightarrow i + 1$ for cut $\#2$ ( $= 0$ for no cut)                          | No  |
| $j \text{ Left Cut}\#2:$                | Column $\#$ to start cut $\# 2$                                                           | No  |
| $j \text{ Right Cut}\#2:$               | Column $\#$ to end cut $\# 2$                                                             | No  |
| $i\text{Cut}\#3:$                       | Bond $i \leftrightarrow i + 1$ for cut $\#3$ ( $= 0$ for no cut)                          | No  |
| $j \text{ Left Cut}\#3:$                | Column $\#$ to start cut $\# 3$                                                           | No  |
| $j \text{ Right Cut}\#3:$               | Column $\#$ to end cut $\# 3$                                                             | No  |
| $j\text{TwtBrd}\#1:$                    | Perform twist/braid on inter-slice bonds between slices $j$ and $j + 1$ ( $= 0$ for none) | No  |
| $\text{Twist}\#1:$                      | Perform a twist on all intra-slice bonds between columns $j$ and $j + 1$                  | No  |
| $\text{Braid}\#1:$                      | Perform random braid of ribbons between columns $j$ and $j + 1$                           | Yes |
| $j\text{TwtBrd}\#2:$                    | Perform twist/braid on inter-slice bonds between slices $j$ and $j + 1$ ( $= 0$ for none) | No  |
| $\text{Twist}\#2:$                      | Perform a twist on all intra-slice bonds between columns $j$ and $j + 1$                  | No  |
| $\text{Braid}\#2:$                      | Perform random braid of ribbons between columns $j$ and $j + 1$                           | Yes |

The subsections below describe in greater detail the construction of the quantum dragon graphs. A screen shot is provided in Fig. 6.

### A. cdf3: Carbon-based dragon graphs: Hamiltonian

The simplest associated Hamiltonian to make all of these devices into a quantum dragon, namely devices with transmission  $\mathcal{T}(E) = 1$  for  $-2 < E < 2$  and exhibiting **order amidst disorder**, is the Hamiltonian with:

- All inter-slice bonds to be  $t_{i,j;i,j+1} = 1$ ,
- If the intra-slice bonds are present all  $t_{i,j;i+1,j} = 1$ ,
- The bonds connecting the leads to the device are all equal (we use a uniform  $\vec{v}_{\text{Dragon}}$ ) and have strength  $1/\sqrt{m}$ ,
- If an atom has one intra-slice bond attached, its on site energy is  $\epsilon_{i,j} = 1$ ,
- If an atom has no intra-slice bond attached, its on site energy is  $\epsilon_{i,j} = 0$ ,
- If a twist is present, the associated intra-slice hopping changes sign.

With this Hamiltonian, the quantum dragon nanodevice can easily be considered as being based on proper manipulations of a GNR. The assigned values for the hopping and on site energies are indeed exactly those which easily allow the traditional armchair single-walled carbon nanotube or zigzag GNR able to be solved using the similarity transformation method described in the main text. Note, however, that the graph plot uses the Mathematica algorithm `GraphPlot3D` using the option "`SpringElectricalEmbedding`", and as such is not associated necessarily with the location of carbon atoms in an actual carbon-based nanodevice.

### B. cdf3: Carbon-based dragon graphs: Ribbons, Twists, and Braiding

Following cuts and/or changing the fraction of intra-slice bonds to a non-zero value, it is possible to obtain up to  $m$  different ribbons. We count a new ribbon for twisting/braiding purposes if there is a sequence of four or more values along the direction of electron flow that have missing intra-slice bonds. Let  $M_{\text{ribbon}}$  be the number of ribbons between the chosen slices. The bonds may be missing because of the 2D hexagonal graph, the three cuts one can put on by hand, or setting some random intra-slice bonds to be missing.

The twists, if desired using `Twist#`, are performed between two slices. This is accomplished by forming a  $m \times m$  permutation matrix  $\mathbf{U}_{\text{Twist}}$  which is a matrix sum of  $M_{\text{ribbon}}$  unitary anti-diagonal matrices which each have the size of the number of atoms in the ribbon. For example, if  $M_{\text{ribbon}} = 3$  and the ribbons have widths 2, 4, 3 then the permutation matrix is

$$\mathbf{U}_{\text{Twist}} = \begin{pmatrix} 0 & 1 & 0 & 0 & 0 & 0 & 0 & 0 & 0 \\ 1 & 0 & 0 & 0 & 0 & 0 & 0 & 0 & 0 \\ 0 & 0 & 0 & 0 & 0 & 1 & 0 & 0 & 0 \\ 0 & 0 & 0 & 0 & 1 & 0 & 0 & 0 & 0 \\ 0 & 0 & 0 & 1 & 0 & 0 & 0 & 0 & 0 \\ 0 & 0 & 1 & 0 & 0 & 0 & 0 & 0 & 0 \\ 0 & 0 & 0 & 0 & 0 & 0 & 0 & 0 & 1 \\ 0 & 0 & 0 & 0 & 0 & 0 & 0 & 1 & 0 \\ 0 & 0 & 0 & 0 & 0 & 0 & 1 & 0 & 0 \end{pmatrix}. \quad (3)$$

The twists of a ribbon are all half-twists.

The braids, if desired using **Braid#**, are performed between two slices. This is accomplished by forming a  $m \times m$  permutation matrix  $\mathbf{U}_{\text{Braid}}$  which randomly permutes the order of the ribbons. For example, if  $M_{\text{Ribbon}} = 4$  and the ribbons have widths 2, 4, 3, with the associated atoms

$$\begin{aligned} \text{ribbon\#1 :} & \iff 1, 2 \\ \text{ribbon\#2 :} & \iff 3, 4, 5, 6 \\ \text{ribbon\#3 :} & \iff 7, 8, 9 \end{aligned} \tag{4}$$

then a possible non-trivial braid permutation matrix with the ribbons in order 3, 2, 1 is

$$\mathbf{U}_{\text{Braid}} = \begin{pmatrix} 0 & 0 & 0 & 0 & 0 & 0 & 1 & 0 & 0 \\ 0 & 0 & 0 & 0 & 0 & 0 & 0 & 1 & 0 \\ 0 & 0 & 0 & 0 & 0 & 0 & 0 & 0 & 1 \\ 1 & 0 & 0 & 0 & 0 & 0 & 0 & 0 & 0 \\ 0 & 1 & 0 & 0 & 0 & 0 & 0 & 0 & 0 \\ 0 & 0 & 1 & 0 & 0 & 0 & 0 & 0 & 0 \\ 0 & 0 & 0 & 1 & 0 & 0 & 0 & 0 & 0 \\ 0 & 0 & 0 & 0 & 1 & 0 & 0 & 0 & 0 \\ 0 & 0 & 0 & 0 & 0 & 1 & 0 & 0 & 0 \end{pmatrix}. \tag{5}$$

The intra-slice matrix at the twist/braid location is

$$\mathbf{B} = -\mathbf{U}_{\text{Braid}} \mathbf{U}_{\text{Twist}}. \tag{6}$$

Note the call to **GraphPlot3D** only inputs the adjacency matrix for the graph. Therefore, it does not distinguished between whether the twists are clockwise or counter-clockwise half twists. Furthermore, sometimes two twists or braids may undo each other, or be undone by a changing what is the inside or outside of a curved surface.

### C. cdf3: Carbon-based dragon graphs: Caution

The one caution for this **.cdf** is one may get out-of-bounds values for some pop-up variables. This happens when you decrease  $\ell$  or  $m$  and the pop-up menu items are out of bounds. The pop-up values are out of bounds if the display is blank, rather than a number. This can be avoided by re-setting all values of the other pop-up menus to values within the range before changing  $\ell$  or  $m$ . Note except for  $\ell$  and  $m$ , setting all numerical pop-up values to zero means they are all within the allowed range.

```

l = # slices      100      m = # atoms per slice  32
# left lead atoms  3        # right lead atoms  2
                                frac intra- bonds = 0    0.

# Left to sew      50        # Right to sew      50

    i Cut#1      8          j Left Cut#1      25        j Right Cut#1      75
    i Cut#2     16          j Left Cut#2      65        j Right Cut#2     98
    i Cut#3     24          j Left Cut#3      25        j Right Cut#3      75

j TwtBrd#1      8          Twist#1      True          Braid#1      True
j TwtBrd#2     66          Twist#2      True          Braid#2      True

```

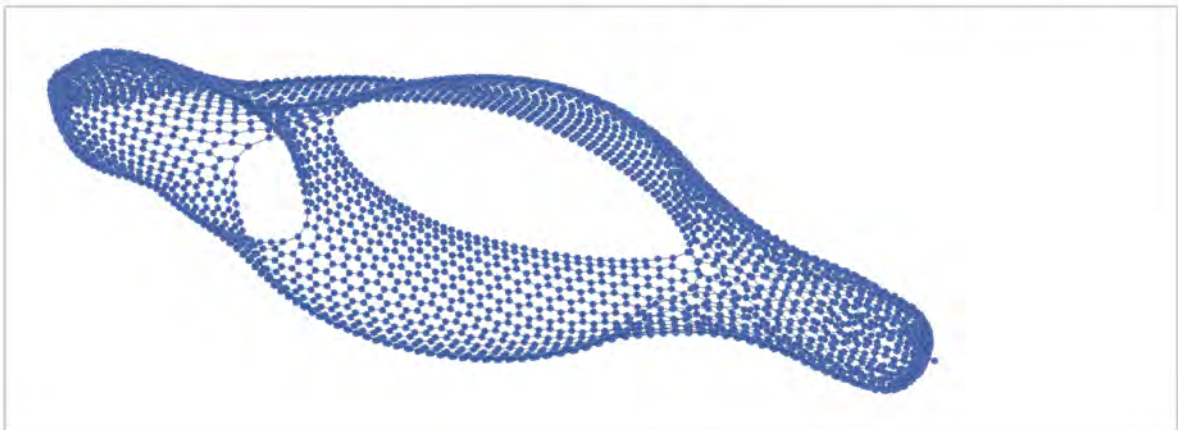

Figure 6. A screenshot of the program `Dragon_cdf3_Cdevice.cdf`, showing possible input and the associated carbon-based (2D hexagonal graph) nano-device.

#### IV. CDF#4: ORDER AMIDST DISORDER

The goal of this `.cdf` program is to demonstrate **order amidst disorder**.

Order amidst disorder is demonstrated here using 2D graphs. The graphs may be 2D hexagonal, 2D rectangular, 2D square-octagonal, or select combinations of them. Two combination graphs are shown in Fig. 7.

It is possible to *just play* with the program.

A further understanding can be obtained using the two tables in subsection A describing the variables. The checkbox variables are described in Table VI, and the pop-up variables in Table VII. The remaining subsections need only be read if the reader wants a greater understanding of the construction of the quantum dragon nanodevices.

All devices are quantum dragon nanodevices if  $\delta = 0$ . As such they all have  $\mathcal{T}(E) = 1$  for all  $-2 < E < 2$ , as seen if this transmission is plotted. Furthermore, they all have **order amidst disorder (OaD)**, as best seen when the  $\text{LDOS}_{i,j}(E)$  is plotted (and OaD is often also seen in the local bond currents).

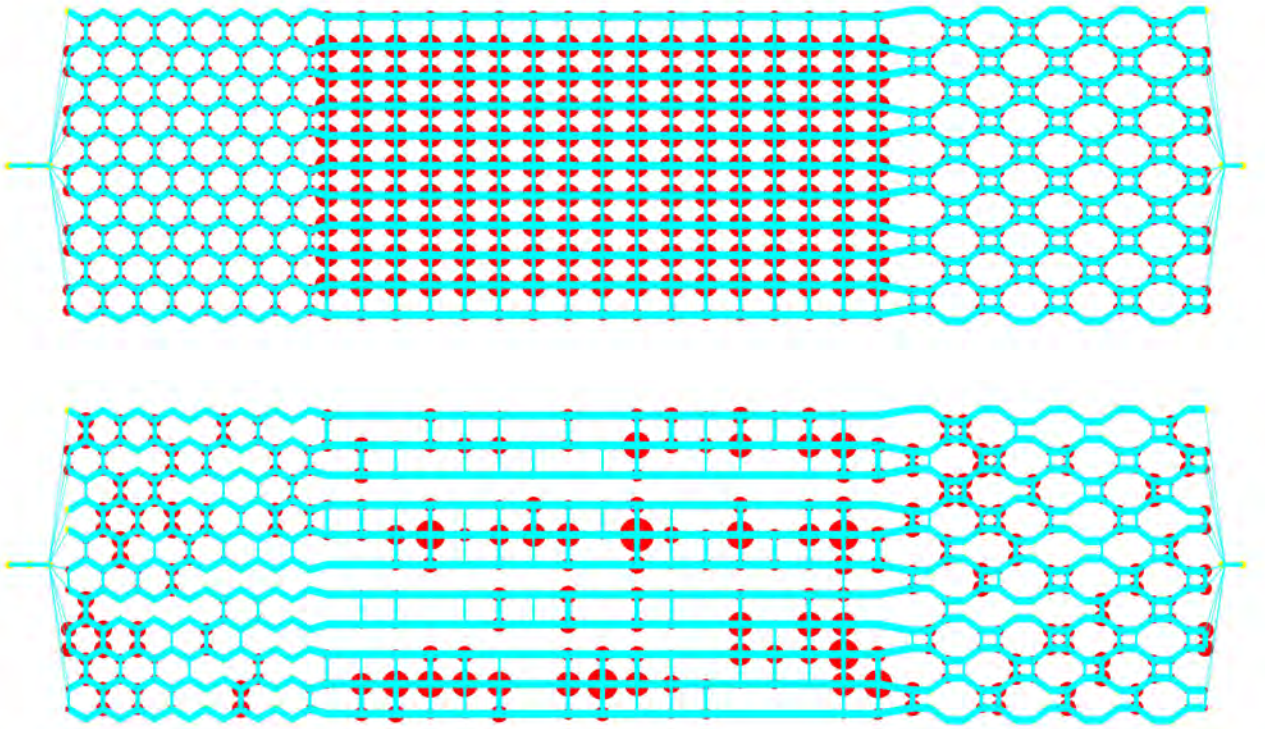

Figure 7. Two sample 2D graphs from `Dragon_cdf4_0aD.cdf` of quantum dragons, so they exhibit **order amidst disorder** and  $\mathcal{T}(E) = 1$  for  $-2 < E < 2$ . Here  $\ell = 50$  and  $m = 11$ , and to better show the graph the bonds (cyan cylinders, with radii proportional to the hopping strength  $t_{i,j;i',j'}$ ) are depicted on top of the vertices (red disks, with radii proportional to the on site energies  $\epsilon_{i,j}$ ). The yellow disks represent  $\epsilon_{i,j} = 0$ , which is also the case for the lead atoms. The graphs have the left-hand side as a 2D hexagonal graph, the middle as a rectangular graph, and the right-hand side as a square-octagonal graph. The top graph is uniform, with all  $t_{i,j;i',j'} = 1$ . The bottom graph has three cuts, and 20% of the intra-slice bonds are set to zero, and  $\Delta_{\text{Dragon},At} = 0.5$ . These graphs have no nnn bonds. See the text in Sec. IV for a complete description.

### A. cdf4: OaD: Manipulate Variable Description

Table VI. Description of the `Dragon_cdf4_OaD.cdf` seven check-box controls.

|     |                                      |                                                                                                                                                                                                                                                                                                                                                               |
|-----|--------------------------------------|---------------------------------------------------------------------------------------------------------------------------------------------------------------------------------------------------------------------------------------------------------------------------------------------------------------------------------------------------------------|
| T-F | New Dragon $\mathcal{H}$             | If checked a new device Hamiltonian $\mathcal{H}_{\text{Dragon}}$ is calculated when popup values are changed. The Hamiltonian is set to the dragon condition, so the it shows <b>order amidst disorder</b> and $\mathcal{T}(E) = 1$ for $-2 < E < 2$ .<br>A new Hamiltonian is also calculated whenever popup menus change values for either $\ell$ or $m$ . |
| T-F | New $\delta$ disorder                | If unchecked and re-checked new uncorrelated random disorder with strength $\delta$ is formed.                                                                                                                                                                                                                                                                |
| T-F | <b>Plot/Eval:</b> Device             | Plot, if checked, as a ball-and-stick model the device Hamiltonian $\mathcal{H}_\ell$ in physical space                                                                                                                                                                                                                                                       |
| T-F | <b>Plot/Eval:</b> $\mathcal{T}(E)$   | Calculate and plot, if checked, $\mathcal{T}(E)$ for the select number of energies.                                                                                                                                                                                                                                                                           |
| T-F | <b>Plot/Eval:</b> Graph              | Plot if checked the graph, using <code>GraphPlot[H]</code> .                                                                                                                                                                                                                                                                                                  |
| T-F | <b>Plot/Eval:</b> LDOS $_{i,j}(E)$   | If checked the local density of states at each site for the chosen energy $E$ is plotted.                                                                                                                                                                                                                                                                     |
| T-F | <b>Plot/Eval:</b> $I_{i,j;i',j'}(E)$ | If checked a plot of the local bond currents at the chosen energy $E$ is shown.                                                                                                                                                                                                                                                                               |

An example of the output showing **order amidst disorder** is shown in Fig. 8.

### B. cdf4: OaD: Graph Generation

All graphs allow only nearest-neighbor (nn) intra-slice bonds, but if  $\Delta_{\text{Dragon}, Bx}$  is non-zero allows next-nearest-neighbor (nnn) inter-slice bonds.

The three parameters  $P_{\text{hex}}$ ,  $P_{\text{sq}}$ , and  $P_{\text{sqOct}}$  give respectively the ratio (on average) of the left-hand hexagonal sub-graph, the middle square sub-graph, and the right-hand side square-octagonal sub-graph. The graphs are depicted both as a device and as a graph, provided the appropriate boxes are checked. The vertices of graph are denoted by  $\epsilon_{i,j}$ , with  $i = 1, 2, \dots, m$  and  $j = 1, 2, \dots, \ell$ .

It is possible to place a number of cuts on the graph. These cuts are at a random location between  $i \leftrightarrow i + 1$ , with the start of the cut at a value  $j_{\text{start}}$  randomly drawn from the left-hand side of the graph and the end of the cut at a value  $j_{\text{end}}$  drawn from the right-hand side of the graph. The cuts are for both intra-slice nn bonds and inter-slice nnn bonds, since the cuts are horizontal.

The variable `fraction intra-bonds=0`) has intra-slice bonds cut with this probability.

### C. cdf4: OaD: Intra-slice Matrices $\mathbf{A}_j$

The random values of the intra-slice hopping are chosen uniformly at random with  $t_{i,j;i+1,j} \in [1 - \Delta_{\text{Dragon}, At}, 1 + \Delta_{\text{Dragon}, At}]$ . The values are chosen in an uncorrelated fashion, so every intra-slice bond has its own draw of the random value.

The quantum dragon condition is satisfied for the intra-slice submatrices (written here for  $m = 6$ )

$$\mathbf{A}_j = \begin{pmatrix} \epsilon_{1,j} & -t_{1,j;2,j} & 0 & 0 & 0 & 0 \\ -t_{1,j;2,j}^* & \epsilon_{2,j} & -t_{2,j;3,j} & 0 & 0 & 0 \\ 0 & -t_{2,j;3,j}^* & \epsilon_{3,j} & -t_{3,j;4,j} & 0 & 0 \\ 0 & 0 & -t_{3,j;4,j}^* & \epsilon_{4,j} & -t_{4,j;5,j} & 0 \\ 0 & 0 & 0 & -t_{4,j;5,j}^* & \epsilon_{5,j} & -t_{5,j;6,j} \\ 0 & 0 & 0 & 0 & -t_{5,j;6,j}^* & \epsilon_{6,j} \end{pmatrix} \quad (7)$$

Table VII. Description of the `Dragon_cdf4_OaD.cdf` sixteen popup variable controls. Note  $i \pm 1$  is to be read including free boundary conditions, so  $i+1 \rightarrow 1$  for  $i=m$  and  $i-1 \rightarrow m$  for  $i=1$ , but with no bond present.

|                                          |                                                                                                                                                                                                                         |
|------------------------------------------|-------------------------------------------------------------------------------------------------------------------------------------------------------------------------------------------------------------------------|
| $P_{\text{hex}}$ :                       | Probability for length of left-hand side graphene nanoribbon (2D hexagonal graph)                                                                                                                                       |
| $P_{\text{sqr}}$ :                       | Probability for length of middle section for square graph                                                                                                                                                               |
| $P_{\text{sqOct}}$ :                     | Probability for length of right-hand side square-octagonal graph                                                                                                                                                        |
| $\ell = \# \text{ slices}$ :             | Number of slices $\ell$ .                                                                                                                                                                                               |
| $m = \# \text{ atoms per slice}$ :       | Number of atoms per slice, $m$ .                                                                                                                                                                                        |
| $\Delta_{\text{Dragon},At}$ :            | The intra-slice bond strengths are chosen uniformly at random<br>with $t_{i,j;i+1,j} \in [1 - \Delta_{\text{Dragon},At}, 1 + \Delta_{\text{Dragon},At}]$ .                                                              |
| $\Delta_{\text{Dragon},Bx}$ :            | The inter-slice bond strengths are chosen uniformly at random. Let $r_j \in [1 - \Delta_{\text{Dragon},B}, 1]$ ,<br>which sets strength of nnn bonds<br>(nn bonds as described in the text to satisfy dragon condition) |
| $\delta$ :                               | Uncorrelated additional on site disorder, added to the dragon on site energy via<br>$\epsilon_{i,j} \rightarrow \epsilon_{i,j} + \delta_{i,j}$ with the random value $\delta_{i,j} \in [-\delta, \delta]$               |
| $\Delta_{\text{vDragon}}$ :              | Dragon vector at first slice chosen uniformly at random in $[1 - \Delta_{\text{vDragon}}, 1 + \Delta_{\text{vDragon}}]$<br>and then normalized (for other slices see text)                                              |
| $\# \text{ cuts}$ :                      | Number of cuts along the electron flow axis, with the cut randomly chosen between<br>$i_{\text{cut, left}} \in [1, \ell/2]$ and $i_{\text{cut, right}} \in [\ell/2, 1]$ .                                               |
| <code>fraction intra- bonds = 0</code> : | Fraction of intra-slice bonds set uniformly at random to zero (before the cuts are put in)                                                                                                                              |
| $P_{\text{stop1}}$ :                     | For calculating intra-slice nnn bonds: probability 'string' stops after one atom                                                                                                                                        |
| $P_{\text{stop2}}$ :                     | For calculating intra-slice nnn bonds: probability 'string' stops after two atoms                                                                                                                                       |
| $P_{\text{stopO}}$ :                     | For calculating intra-slice nnn bonds: probability long 'string' stops here                                                                                                                                             |
| $\# E \text{ points}$ :                  | Number of energy points to calculate, from $E_{\text{min}} = -1.999$ to $E_{\text{max}} = 1.999$                                                                                                                        |
| $E \text{ for LDOS and currents}$ :      | Energy to use to calculate $\text{LDOS}_{i,j}(E)$ and $I_{i,j;i',j'}(E)$                                                                                                                                                |

by insisting that the on site energies  $\epsilon_{i,j}$  are set so

$$\mathbf{A} \vec{v}_{\text{Dragon},j} = \vec{0}. \quad (8)$$

Here  $\vec{v}_{\text{Dragon},j}$  is the dragon vector associated with slice  $j$ , and all elements are chosen to be positive (not zero or negative) and the vector is normalized so  $\vec{v}_{\text{Dragon},j}^\dagger \cdot \vec{v}_{\text{Dragon},j} = 1$ . Any on site energy which is zero, which includes all of the lead atoms, are depicted by yellow disks. Equation (8) means the on site energies are chosen so  $\vec{v}_{\text{Dragon},j}$  is an eigenvector with eigenvalue zero (the chosen zero of energy, which is the on site energy of the lead atoms) of the intra-slice submatrices  $\mathbf{A}_j$ .

Note any intra-slice bond may be missing,  $t_{i,j;i+1,j} = 0$ , when the graph is generated. This happens if:

- The bond is not present in the hexagonal graph or square-octagonal graph.
- The bond is missing (with probability `fraction intra-bonds=0`).
- The bond is one of the bonds cut since the parameter `# cuts` is not zero.

#### D. cdf4: OaD: Dragon vectors, $\vec{v}_{\text{Dragon},j}$

Unlike in most of the main paper where we studied mainly uniform dragon vectors and assumed the dragon vectors were the same for every slice, here we allow the dragon vectors to have randomness and allow them to be somewhat

different at every slice. Therefore, slice  $j$  will have an associated dragon vector  $\vec{v}_{\text{Dragon},j}$ .

The values of  $\vec{v}_{\text{Dragon},1}$  at slice  $j = 1$  is found using the parameter  $\Delta v_{\text{Dragon}}$ . Each of the  $m$  elements of  $\vec{v}_{\text{Dragon},1}$  is set to a random value chosen in  $[1 - \Delta v_{\text{Dragon}}, 1 + \Delta v_{\text{Dragon}}]$ , and then the vector is normalized so  $\vec{v}_{\text{Dragon},1}^\dagger \cdot \vec{v}_{\text{Dragon},1} = 1$ .

The remaining  $\vec{v}_{\text{Dragon},j}$  for  $j \geq 2$  use the value for  $\vec{v}_{\text{Dragon},j-1}$  and the random values of  $\mathbf{B}_{j-1,j}$  as described in the next subsection.

A uniform  $\vec{v}_{\text{Dragon},j}$  for every slice  $j$  can be obtained by setting  $\Delta v_{\text{Dragon}} = 0$  and ensuring all  $\mathbf{B}_{j,j+1}$  inter-slice matrices are symmetric.

The construction described ensures every element of all  $\vec{v}_{\text{Dragon},j}$  are positive (i.e. not zero or negative).

#### E. cdf4: OaD: Inter-slice Matrices $\mathbf{B}_{j,j+1}$

The  $m \times m$  inter-slice matrices  $\mathbf{B}_{j,j+1}$  (written here for  $m = 6$ ) have the form

$$\mathbf{B}_{j,j+1} = \begin{pmatrix} -t_{1,j;1,j+1} & -t_{1,j;2,j+1} & 0 & 0 & 0 & 0 \\ -t_{1,j;2,j+1}^* & -t_{2,j;2,j+1} & -t_{2,j;3,j+1} & 0 & 0 & 0 \\ 0 & -t_{2,j;3,j+1}^* & -t_{3,j;3,j+1} & -t_{3,j;4,j+1} & 0 & 0 \\ 0 & 0 & -t_{3,j;4,j+1}^* & -t_{4,j;4,j+1} & -t_{4,j;5,j+1} & 0 \\ 0 & 0 & 0 & -t_{4,j;5,j+1}^* & -t_{5,j;5,j+1} & -t_{5,j;6,j+1} \\ 0 & 0 & 0 & 0 & -t_{5,j;6,j+1}^* & -t_{6,j;6,j+1} \end{pmatrix}. \quad (9)$$

They need not be Hermitian matrices. The method to calculate the  $\mathbf{B}_{j,j+1}$  is rather complicated as detailed in the description that follows. The important thing is that  $\mathbf{B}_{j,j+1}$  when it undergoes a singular value decomposition (SVD) has the smallest singular value  $\sigma_1 = -1$  (the value of the hopping between lead atoms), with the associated left-singular vector  $\vec{v}_{\text{Dragon},j}$  and associated right-singular vector  $\vec{v}_{\text{Dragon},j+1}$ .

The detailed algorithms for forming the inter-slice matrices  $\mathbf{B}_{i,j;i',j+1}$  are presented. The important thing, with the SVD decomposition of  $\mathbf{B}_{i,j;i',j+1}$ , are to satisfy the constraints:

- The smallest singular value of  $\sigma_1 = -1$  (the hopping term between the lead atoms)
- All elements of  $\mathbf{B}_{i,j;i',j+1}$  are negative or zero (chosen so all bonds have the same sign)
- Only nn and nnn inter-slice bonds are present
- the left-singular vector of  $\mathbf{B}_{i,j;i',j+1}$  associated with the singular value  $\sigma_1$  is  $\vec{v}_{\text{Dragon},j}$
- the right-singular vector of  $\mathbf{B}_{i,j;i',j+1}$  associated with the singular value  $\sigma_1$  is  $\vec{v}_{\text{Dragon},j+1}$

The construction of  $\mathbf{B}_{i,j;i',j+1}$  is defined below in order to satisfy these constraints. Using the parameter  $\Delta v_{\text{Dragon}}$  the elements of the first (left-most) dragon vector is set by choosing elements uniformly at random in  $[1 - \Delta v_{\text{Dragon}}, [1 + \Delta v_{\text{Dragon}}]]$ .

Each inter-slice matrix independently has nnn inter-slice bonds set to zero by the algorithm:

- Start at  $i = 0$  and proceed until  $i = m - 1$
- The initial string length is  $l_{\text{string}} = 0$ 
  - \* Set  $i \rightarrow i + 1$ , and generate uniformly a random number  $r \in [0, 1]$
  - If  $l_{\text{string}} = 0$ , set  $l_{\text{string}} = 1$  and go to \*
  - If  $l_{\text{string}} = 1$ 
    - ▷ If  $r \leq P_{\text{stop},1}$  cut the nnn bond  $t_{i,j;i+1,j} = 0$ , set  $l_{\text{string}} = 0$ , and go to \*
    - ▷ If  $r > P_{\text{stop},1}$  set  $l_{\text{string}} = 2$  and go to \*
  - If  $l_{\text{string}} = 2$ 
    - ▷ If  $r \leq P_{\text{stop},2}$  cut the nnn bond  $t_{i,j;i+1,j} = 0$ , set  $l_{\text{string}} = 0$ , and go to \*
    - ▷ If  $r > P_{\text{stop},2}$  set  $l_{\text{string}} = 3$  and go to \*
  - If  $l_{\text{string}} > 2$ 
    - ▷ If  $r \leq P_{\text{stop},O}$  cut the nnn bond  $t_{i,j;i+1,j} = 0$ , set  $l_{\text{string}} = 0$ , and go to \*
    - ▷ If  $r > P_{\text{stop},O}$  set  $l_{\text{string}} = l_{\text{string}} + 1$  and go to \*

Some additional inter-slice nnn bonds  $t_{i,j;i\pm 1,j+1}$  are set to zero due to the cuts, potentially cutting some strings. The strengths of the nnn inter-slice bonds between slices  $j$  and  $j + 1$  are then chosen such that:

- If  $l_{\text{string}} = 1$  at index ( $i$ ):
  - There are no nnn intra-slice bonds
  - Set both nnn bonds to zero,  $t_{i,j;i\pm 1,j+1} = 0$
  - Set the nn intra-slice bond to  $t_{i,j;i,j+1} = 1$
  - Set the  $i^{\text{th}}$  element of  $\vec{v}_{\text{Dragon},j+1} = \vec{v}_{\text{Dragon},j}$
- If  $l_{\text{string}} = 2$  at indices ( $i$ ) and ( $i + 1$ ):
  - Form the  $2 \times 2$  unitary matrix  $\mathbf{U}_{2 \times 2} = \begin{pmatrix} \cos(\theta) & \sin(\theta) \\ \sin(\theta) & -\cos(\theta) \end{pmatrix}$  with the angle  $\theta$  determined from the normalized  $2 \times 2$  vector formed by the  $i^{\text{th}}$  and  $(i + 1)^{\text{st}}$  elements of  $\vec{v}_{\text{Dragon},j}$ ; Since the elements of  $\vec{v}_{\text{dragon}}$  are all positive, the angle  $\theta$  is in the first quadrant

- Form the  $2 \times 2$  unitary matrix  $\mathbf{V}_{2 \times 2} = \begin{pmatrix} \cos(\phi) & \sin(\phi) \\ \sin(\phi) & -\cos(\phi) \end{pmatrix}$  with the angle  $\phi$  chosen uniformly at random with  $\phi \in [\frac{\pi}{12}, \frac{\pi}{2} - \frac{\pi}{12}]$ , which ensures the elements of the new dragon vector are all positive,
  - Form the  $2 \times 2$  diagonal matrix  $\mathbf{W}_{2 \times 2} = \begin{pmatrix} \sigma_1 & 0 \\ 0 & \sigma_2 \end{pmatrix}$  with the singular values  $\sigma_1 = 1$  and a random value chosen uniformly such that  $\sigma_2 \leq \sigma_1$  and the matrix  $\mathbf{U}_{2 \times 2} \mathbf{W}_{2 \times 2} \mathbf{V}_{2 \times 2}$  has all four elements non-negative, this is accomplished by choosing  $\sigma_2$  uniformly at random between  $-\min(\tan(\theta) \tan(\phi), \cot(\theta) \cot(\phi))$  and  $\min(\tan(\theta) \cot(\phi), \cot(\theta) \tan(\phi))$ ,
  - Set the respective  $2 \times 2$  submatrix of  $\mathbf{B}_{j,j+1}$  to be the matrix  $-\mathbf{U}_{2 \times 2} \mathbf{W}_{2 \times 2} \mathbf{V}_{2 \times 2}$ ; all elements of this  $2 \times 2$  sub-matrix of  $\mathbf{B}_{j,j+1}$  will then be negative,
  - Set the elements  $i$  and  $i + 1$  of  $\vec{v}_{\text{Dragon},j+1}$  to  $\begin{pmatrix} \cos(\phi) \\ \sin(\phi) \end{pmatrix}$
- If  $l_{\text{string}} > 2$  at indices  $(i)$  to  $(i + l_{\text{string}} - 1)$ 
  - Form the Hermitian tri-diagonal matrix  $\mathbf{H}_{\text{string}}$  of size  $l_{\text{string}} \times l_{\text{string}}$ 
    - ▷ The nnn inter-slice bonds along the upper diagonal are chosen uniformly at random in  $t_{i,j;i+1,j+1} \in [0, \Delta_{\text{Dragon},Bx}]$
    - ▷ The nnn inter-slice bonds along the lower diagonal are chosen so  $\mathbf{H}_{\text{string}}$  is Hermitian, namely  $t_{i,j;i+1,j+1} = t_{i+1,j;i,j+1}$
    - ▷ The nn bonds are chosen such that the length  $l_{\text{string}}$  vector  $\vec{x}_{\text{string}}$  formed by associated elements of  $\vec{v}_{\text{Dragon},j}$  satisfies  $\mathbf{H}_{\text{string}} \vec{x}_{\text{string}} = \vec{x}_{\text{string}}$ . In other words  $\vec{x}_{\text{string}}$  is an eigenvector of  $\mathbf{H}_{\text{string}}$  with eigenvalue  $+1$  (the strength of the hopping in the uniform leads, chosen to be our unit of energy). Note since all elements of  $\vec{v}_{\text{Dragon}}$  are non-zero this construction is always possible.
  - Set the appropriate  $l_{\text{string}} \times l_{\text{string}}$  submatrix of  $\mathbf{B}_{j,j+1}$  to  $-\mathbf{H}_{\text{string}}$
  - Set the elements  $i$  to  $i + l_{\text{string}} - 1$  of  $\vec{v}_{\text{Dragon},j+1}$  to the respective elements of  $\vec{v}_{\text{Dragon},j}$
- Normalize the vector  $\vec{v}_{\text{Dragon},j+1}$

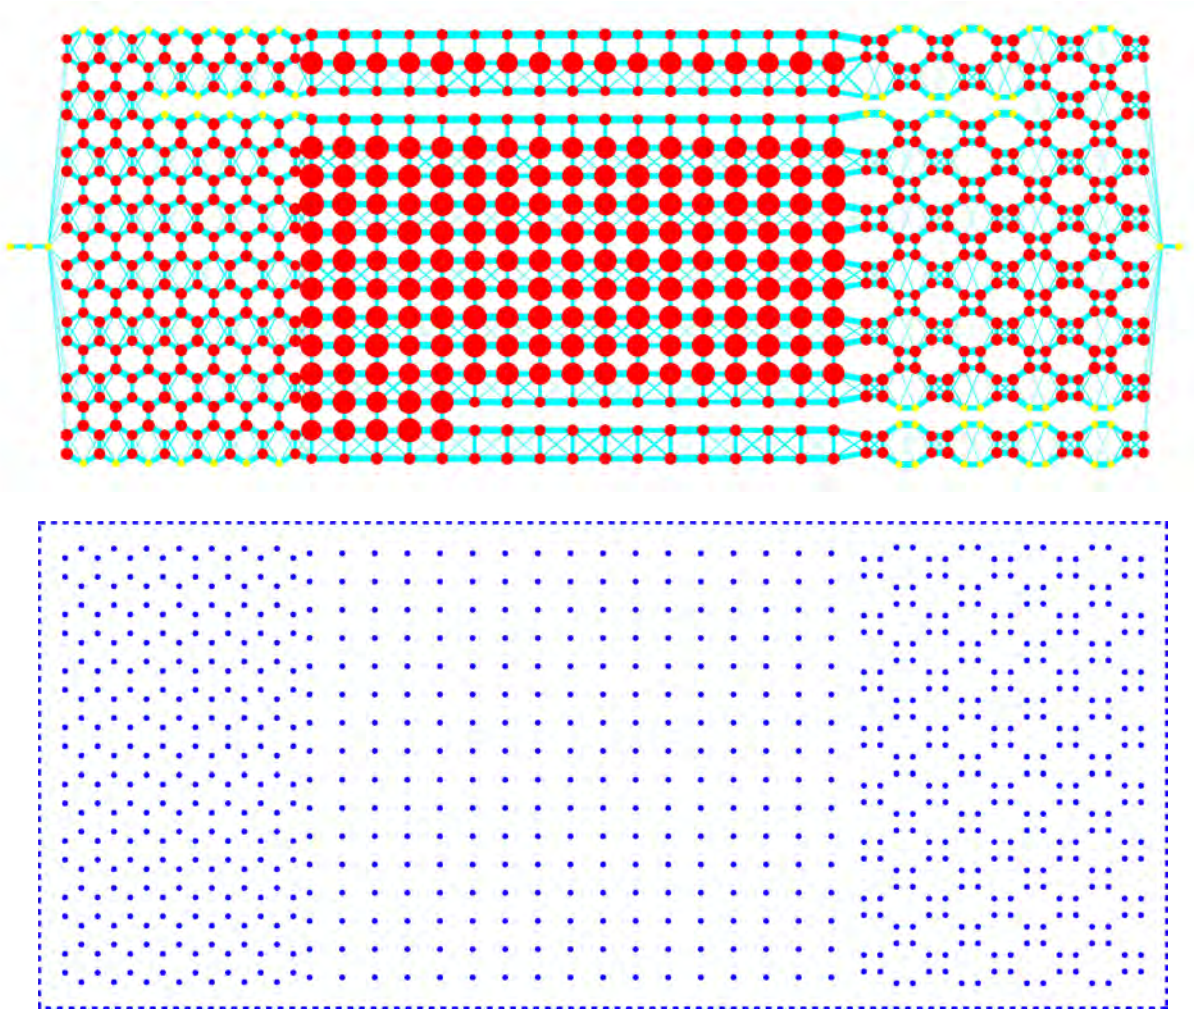

Figure 8. Example device and  $\text{LDOS}_{i,j}(E)$  from `Dragon_cdf4_0aD.cdf`. This illustrates **order amidst disorder**, as the  $\ell = 50$  and  $m = 16$  disordered nanodevice on the top is disordered. It is comprised of the left third a 2D hexagonal graph, middle third a rectangular graph, right third a square-octagonal graph. The graph has two cuts, and a uniform  $\vec{v}_{\text{Dragon}}$  throughout the device. Nevertheless it has an ordered  $\text{LDOS}_{i,j}(E)$ , as seen in the lower blue plot (here at  $E = 1.99$ ). This points out a useful trick, namely since  $\text{LDOS}_{i,j}(E) \propto \frac{1}{\sqrt{4-E^2}}$  once can set the plotting value for  $E$  to be close to the band edge at  $\pm 2$  to make the blue disks showing the LDOS points to be larger. The blue, dashed bounding box is so the user can see there is a plot present in case the LDOS points are too small. See the text in Sec. IV for a complete description.

## V. CDF FIGURES: 3D GRAPHICS OF MAIN TEXT FIGURES

The supplemental material could also contain ten `.cdf` files associated with 3D graphics in the main text. These are associated with various figures, and are listed in Table VIII.

**Unfortunately, these files are not on arXiv!** This is because the files are too large to all fit into the space limitations on arXiv for a single submission. These files will hopefully be present in when the paper is published in the open-access journal to which it has been submitted. If you have need of these files prior to publication, please contact the authors. Most of them are, however, too large to email.

The value of  $N$  gives an idea of how large the file is, and consequently how much processing power and memory is needed for manipulation of the graphic. The same is true for the type of figure, manipulating a graph takes less memory and processing power than manipulating the ball-and-stick model of the device. Some of the quantum dragons are the same as in the figures, while others use different random numbers in the construction associated with the figure while keeping the same values of  $\ell$  and  $m$  and proper graph/Hamiltonian manipulations.

All `.cdf` figures listed are quantum dragons (with an appropriate Hamiltonian for the graphs), and consequently show **order amidst disorder**.

Table VIII. Description of the `.cdf` associated with the figures in the main text.

| File name                   | Text figure      | $N$   | $\ell$ | Same? | Type   |
|-----------------------------|------------------|-------|--------|-------|--------|
| 2020_PRR_dragon_Fig04A.cdf  | Fig. 7(A)        | 3120  | 120    | No    | device |
| 2020_PRR_dragon_Fig04B.cdf  | Fig. 7(B)        | 3120  | 120    | No    | graph  |
| 2020_PRR_dragon_Fig05.cdf   | Fig. 8           | 3120  | 120    | Yes   | graph  |
| 2020_PRR_dragon_Fig06.cdf   | Fig. 9           | 6000  | 120    | Yes   | graph  |
| 2020_PRR_dragon_Fig07A.cdf  | Fig. 10(A)       | 5000  | 100    | No    | graph  |
| 2020_PRR_dragon_Fig07B.cdf  | Fig. 10(B)       | 15000 | 300    | No    | graph  |
| 2020_PRR_dragon_Fig13.cdf   | Fig. 13(C)       | 7200  | 60     | Yes   | device |
| 2020_PRR_dragon_Fig14.cdf   | Fig. 14(B)       | 4100  | 82     | Yes   | graph  |
| 2020_PRR_dragon_Fig15AB.cdf | Fig. 15(A) & (B) | 3456  | 86     | Yes   | device |
| 2020_PRR_dragon_Fig15C.cdf  | Fig. 15(C)       | 3456  | 86     | Yes   | LDOS   |

For an unknown reason, sometimes all or a part of a dragon will disappear ... just keep changing the viewpoint and the dragon should reappear. It is unknown whether this is a bug or a feature, or just a property of dragons.

- 
- [1] Wolfram Research, Inc., Mathematica, Version 12.1, Champaign, IL (2020).
  - [2] M.A. Novotny, Phys. Rev. B **90**, 165103 [14 pages] (2014).
-
